# Supplementary material for: Importance-Aware Data Augmentation for Document-Level Neural Machine Translation
Source: arXiv:2401.15360 source file (2024-01-27)
Supplement: Supplementary file 1 [file 9_appendix.tex]

\section{Method-specific Hyperparameters}
\label{sec:baselines}

\paragraph{Word Dropout (\wdrop)}
We search the optimal $p$ from $[0.1, 0.2, 0.3]$ and report the best results with the replacement probability $p=0.1$.

\paragraph{Word Replacement (\wrep)}
We search for the optimal $p$ from $[0.1, 0.2, 0.3]$ and report the best results with the replacement probability $p=0.1$.

\paragraph{\bpedrop}
The probability of \bpedrop is $0.1$.

\paragraph{\cipheraug}
We use \cipheraug with two keys, so the total size of augmented training data is three times as large as that of the original training data.

% \paragraph{Back-Translation (BT)}
% We only back-translate the original training data and do not introduce any target monolingual corpus for fair comparison.

% \paragraph{Forward-Translation (FT)}
% Like \bt, we only forward-translate the original training data and do not introduce any source monolingual corpus.

% \paragraph{\mixup}
% We search for the optimal $\beta$ from $[0.1, 0.2, 0.3]$ and report the best results with $\beta=0.1$.

\paragraph{\iada}
We set the initial replacement probabilities for both the context and the current sentence to be $p_{\textrm{ctx}}=p_{\textrm{cur}}=0.1$.
We search for the optimal $\alpha$ in \autoref{eq:normalize} from $[0.01, 0.1, 0.2, 0.3]$ and report the best results with $\alpha=0.1$.
